# Supplementary material for: A New Paradigm for Identifying Reconciliation-Scenario Altering Mutations Conferring Environmental Adaptation
Source: arXiv:1912.01934 source file (2019-12-04)
Supplement: Supplementary file 1 [file supplement.tex]

\input{begin}

{\huge \bf Supplemental Material}

\section{Stage 3.1: Coloring the Species and Gene Trees (Optional)} 
\label{sec:coloring}

Our framework can be used to search for {\em different} evolutionary patterns. {\em Some} sought patterns could involve a phenotype of the species. Therefore, we assume that (as a part of the input), each leaf of the Species tree $S$ {\em might} have a color (red or black) to represent its phenotype.
Recall that as part of the input, we are given a function $\mathsf{colors}:L(S)\to \Upsilon$ where $\Upsilon=\{ \mathsf{red},\mathsf{black}\}$.
Initially, for each leaf $\ell\in L(S)$, we define $\mathsf{red}(\ell) = 1$ and $\mathsf{black}(\ell) = 0$ if $\ell$ is red (i.e.~$\mathsf{colors}(\ell)=\mathsf{red}$), and $\mathsf{red}(\ell) = 0$ and $\mathsf{black}(\ell) = 1$ otherwise.  
In the example described in this paper, we use colors as {\em habitat identifiers}.  More precisely, for any leaf $\ell\in L(S)$ representing a species that belongs to an {\em environmental habitat} (soil, water, plants, etc.) we set $\mathsf{black}(\ell)=1$ and $\mathsf{red}(\ell)=0$, and for any leaf $\ell\in L(S)$ representing a species that belongs to a {\em living habitat} (human, animal) we set  $\mathsf{black}(\ell)=0$ and $\mathsf{red}(\ell)=1$.

The goal here is to assign to each vertex $x\in V(S)$ a color $\mathsf{red}(x),\mathsf{black}(x)\in \mathbb{N}_0$ as explained below.\footnote{The standard notation $\mathbb{N}_0$ denotes $\mathbb{N}\cup\{0\}$ where $\mathbb{N}$ is the set of natural numbers.}
 
Now, in postorder, for each internal vertex $x\in V(S)$ with children $y$ and $z$, compute: $\mathsf{red}(x) = \mathsf{red}(y)+\mathsf{red}(z)$, and $\mathsf{black}(x) = \mathsf{black}(y)+\mathsf{black}(z)$.

Additionally, we use $\sigma:L(G)\to L(S)$ to color the vertices of the Gene tree $G$ as follows. Initially, for each leaf $u\in L(G)$, we define $\mathsf{red}(u) = 1$ and $\mathsf{black}(u) = 0$ if $\mathsf{colors}(\sigma(u))=\mathsf{red}$, and $\mathsf{red}(u) = 0$. Otherwise, $\mathsf{black}(u) = 1$. Now, in postorder, for each internal vertex $x\in V(S)$ with children $y$ and $z$, compute: $\mathsf{red}(x) = \mathsf{red}(y)+\mathsf{red}(z)$, and $\mathsf{black}(x) = \mathsf{black}(y)+\mathsf{black}(z)$.

%Next, we will to calculate a weights sum of the colors for each match $(u,x)\in V(\cal H)$, based on the weights we assigned in the previous stage. This is, for each $(u,x)\in V(\cal H)$ we want to calculate $\mathsf{red}(u,x),\ \mathsf{black}(u,x)$, defined as \[ \mathsf{red}(u,x) = \displaystyle{\sum_{i=1} ^{\mathsf{m}(r)} \mathsf{w}(u,x,i)\cdot \mathsf{red}(u,x,i)}, \] and \[ \mathsf{black}(u,x) = \displaystyle{\sum_{i=1} ^{\mathsf{m}(r)} \mathsf{w}(u,x,i)\cdot \mathsf{black}(u,x,i)}. \]

%Finally, for each $x\in V(S)$ we will iterate over all $u\in V(G)$ and sum up $\mathsf{red}(u,x)$, $\mathsf{black}(u,x)$, which will give us an indication of the color of $x$ when considering all $k$-best solutions and their weights. Formally, define \[\mathsf{ERed(x)}=\sum_{u\in V(G)} \mathsf{red}(u,x), \]
%and similarly for $\mathsf{EBlack(x)}$.

%\noindent {\bf Time complexity.} Iterating the hypergraph in $O(|V(\mathcal{H}))|=O(m\cdot n\cdot k)$ time.

\subsection*{Colored Pattern Identification} \label{sec:colored_pattern}
When specifying a pattern $P$ with colors, we need to define the sought pattern. To this end, we will need the following definitions.

\medskip
\noindent{\bf Definitions.} For each hypernode $(u,x,i)\in V(\mathcal{H})$ define $\mathsf{red}(u,x,i)=\mathsf{red}(x)$, $\mathsf{black}(u,x,i)=\mathsf{black}(x)$,  $\mathsf{totalL}(u,x,i)=\mathsf{red}(x)+\mathsf{black}(x)$.
We define $\Pr [\text{red}]=\frac{\textsf{number of red leaves in }S}{\mid L(S)\mid}$, and, similarly $\Pr [\text{black}]=\frac{\textsf{number of black leaves in }S}{\mid L(S)\mid}$.

For a node $(u,x,i)\in V(\mathcal{H})$, we say the it is ``mostly red" if it holds that \[ \sum _{r=\mathsf{red}(u,x,i)+1} ^{\mathsf{totalL}(u,x,i)} \binom {\mathsf{totalL}(u,x,i)}{r} \cdot \Pr [\text{red}]^r\cdot\Pr [\text{black}]^{\mathsf{totalL}(u,x,i)-r} \leq p, \] and is ``mostly black" if it holds that \[ \sum _{r=\mathsf{red}(u,x,i)+1} ^{\mathsf{totalL}(u,x,i)} \binom {\mathsf{totalL}(u,x,i)} r \cdot \Pr [\text{red}]^r\cdot\Pr [\text{black}]^{\mathsf{totalL}(u,x,i)-r} \geq 1- p, \] where $p$ is a predefined probability threshold.  Intuitively, for each hypernode $(u,x,i)\in V(\mathcal{H})$ the formulas above reflect the homogeneity of $S_x$ (the subtree rooted by $x$). As the value of $p$ grows smaller we get a more homogenous subtrees.

For each $\mathsf{EV}\in \{ \mathsf{S}, \mathsf{D},\mathsf{HT} \}$, $\mathsf{color}\in \{\mathsf{red},\mathsf{black} \}$ and $\mathsf{distance}\in \{\mathsf{True},\mathsf{False}\}$, the pattern $(\mathsf{EV},\mathsf{colors},\mathsf{distance})$ is a hypernode $(u,x,i)$ with children $(v,y,j)$ and $(w,z,r)$ (by children we mean that $(u,x,i)\in \mathsf{D}(v,y,j)$ and $(u,x,i)\in \mathsf{D}(w, z,r)$, as defined in Section 4.2), such that both $(v,y,j)$ and $(w,z,r)$ are ``mostly $\mathsf{red}$" or ``mostly $\mathsf{black}$".

\begin{figure}[H]
\begin{center}
\fbox{\includegraphics[scale=0.06]{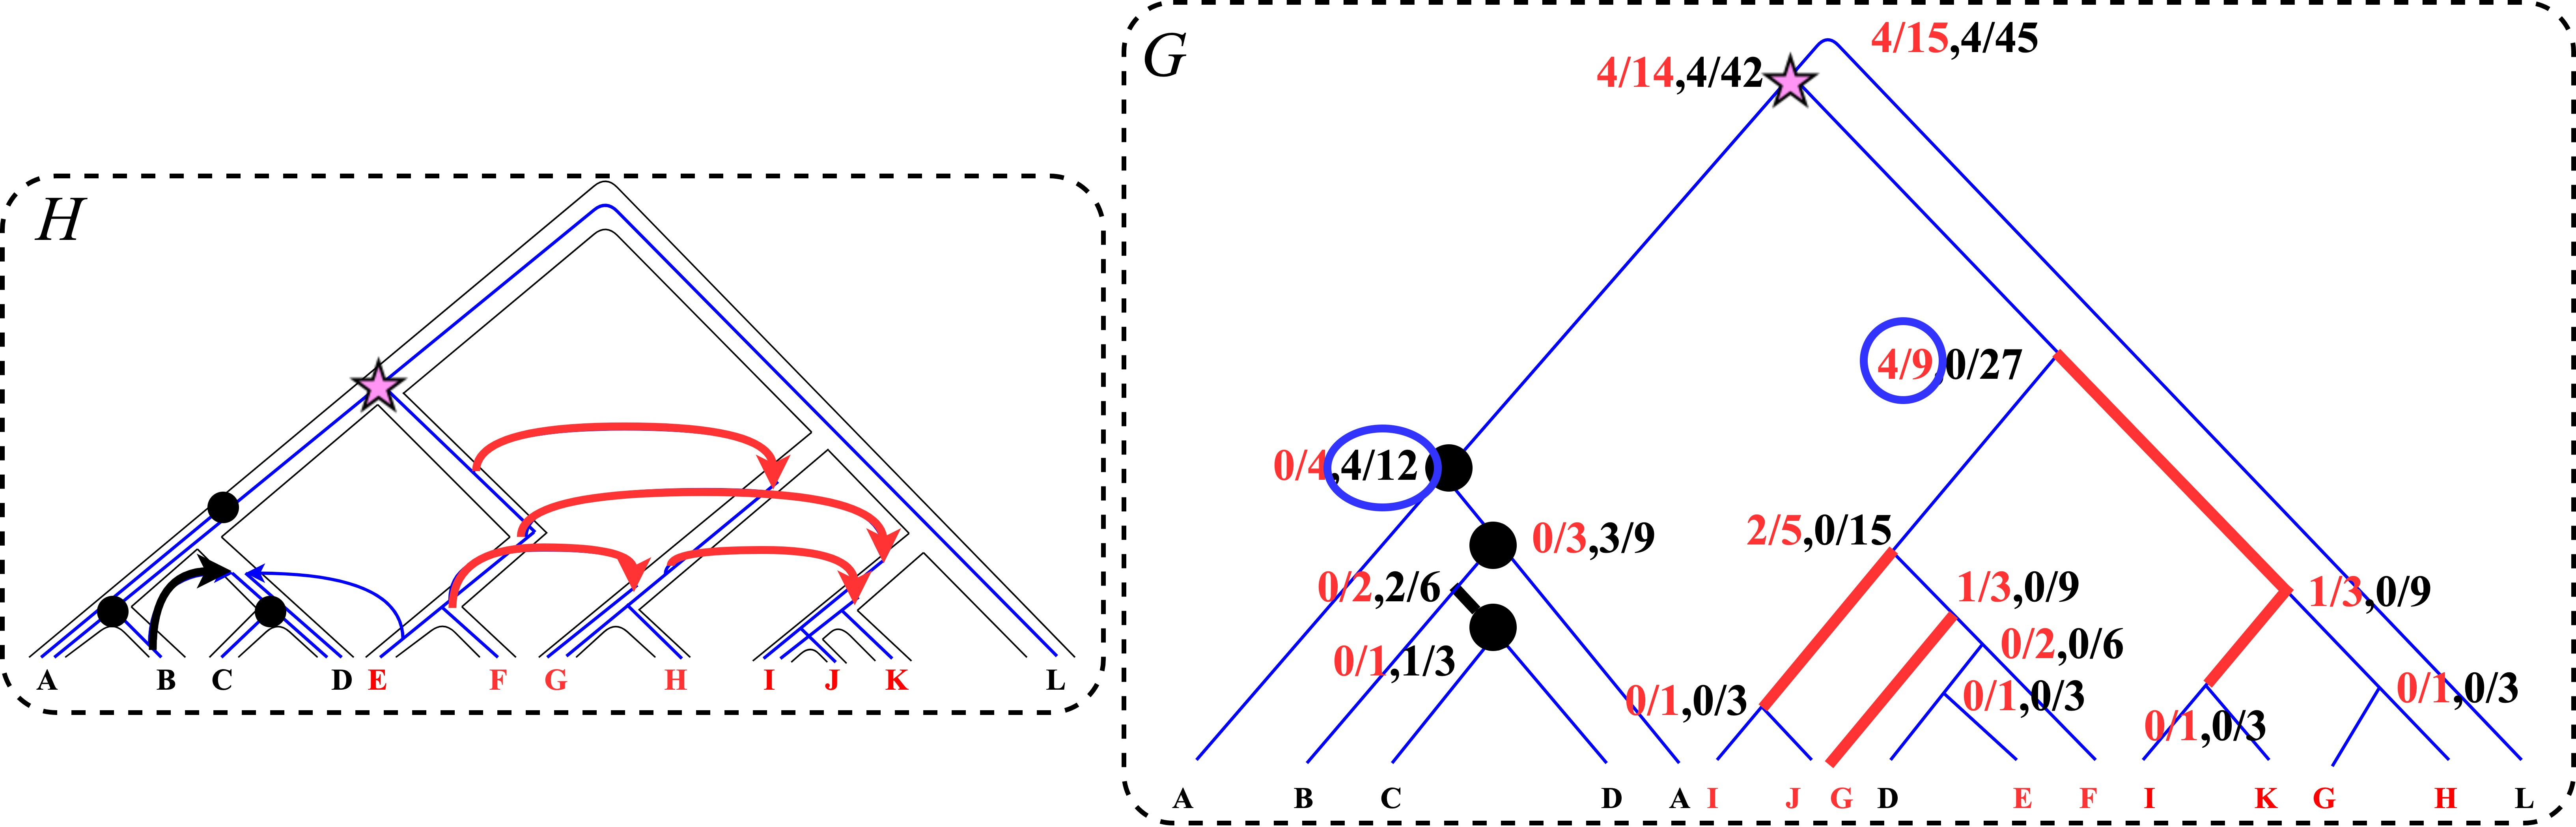} }
\end{center}
\caption{An illustration of the (dual) pattern ($(\{ \mathsf{HT}\} ,\mathsf{red},False)$, $(\{ \mathsf{S,D,HT}\} ,\mathsf{black},False)$), with $k=1$.}
\label{fig:same_color_HT}
\end{figure}

For example, Fig.~8 demonstrates the dual pattern ($(\{ \mathsf{HT}\} ,\mathsf{red},False)$, $(\{ \mathsf{S,D,HT}\} ,\mathsf{black},False)$). $H$ illustrates a hypergraph for $k=1$, and $G$ illustrates a corresponding Gene tree (the corresponding Species tree for this example is not presented in the figure). The colors of the species are the colors of the text, that is, $\mathsf{color}(A)=\mathsf{color}(B)=\mathsf{color}(C)=\mathsf{color}(D)=\mathsf{color}(L)=\mathsf{red}$ and $\mathsf{color}(E)=\mathsf{color}(F)=\mathsf{color}(G)=\mathsf{color}(H)=\mathsf{color}(I)=\mathsf{color}(J)=\mathsf{color}(K)=\mathsf{black}$. Since $k=1$, the hypergraph corresponds to only one optimal solution, thus we use the standard representation for a DLT reconciliation. For more details about this representation, see Fig. 1. The bold red horizontal transfer hyperedges are edges that satisfy our requirements for the first pattern, $(\{\mathsf{HT}\} ,\mathsf{red},False)$, and the bold black hyperedges and hypernodes satisfy the second pattern, $(\{ \mathsf{S,D,HT}\} ,\mathsf{black},False)$. We note that in the figure we marked the hyperedges for simplicity of explanation, where in fact the hypernodes are marked instead. For more details about the identification of the patterns inside the hypergraph, see Substage 1 in Section 4.3.
%a calculation for the vertex $v_1$ for being ``mostly red" for $(u_1,x_1,1)$ is $\sum _{r=3} ^{4} {\binom 4 r} \cdot \left(\frac{1}{2}\right)^r\cdot\left(\frac{1}{2}\right)^{4-r}=0.3125<0.5$ and for $(u_2,x_2,1)$ is the same. Thus, for $p=0.5$ the hypernode representing the match between $u_1$ and $x_1$ will be considered as a pattern satisfying our requirements. On the other hand, the black bold horizontal transfer is not satisfying the requirements, and will not be reported as interesting. In all of our results, we use $p=0.05$.

After identifying the interesting hypernodes, we reflect them to the Gene tree, and each internal vertex is assigned with two scores; one for the pattern $(\{\mathsf{HT}\} ,\mathsf{red},False)$ and the other for the pattern $(\{ \mathsf{S,D,HT}\} ,\mathsf{black},False)$. In the dual pattern mode, we look for the top scoring vertex in the sense of comparing its children's scores. For example, the top scoring vertex in the example in Fig.8 is the vertex marked with a star, since one of its children has the score $4/12$ for the black pattern, and the other has the score of $4/9$ for the red pattern. For more details about the scores, see Substage 2 in Section 4.3.

\section{Naive Algorithm for Hypergraph Construction}
\label{sec:naive_pseoducode}
%!TEX root = Roni_Proposal.tex

In this appendix we present a somewhat naive algorithm to construct the hypergraph that is based on dynamic programming (DP). Here, we present the pseudocode for this algorithm. We proceed with a few clarifications and details that concern the pseudocode. First, we remark that lists of $k$-best solutions are not unique; for example, consider the extreme case where each of the lists returned by SpeciationEvent, DuplicationEvent and HorizontalTransferEvent (in some iteration) consists of $k$ items having the same cost---then, the choice of $k$ items among the combined list consisting of $3k$ items is arbitrary.

\begin{figure}[htbp]
\begin{center}\fbox{\includegraphics[scale=0.15]{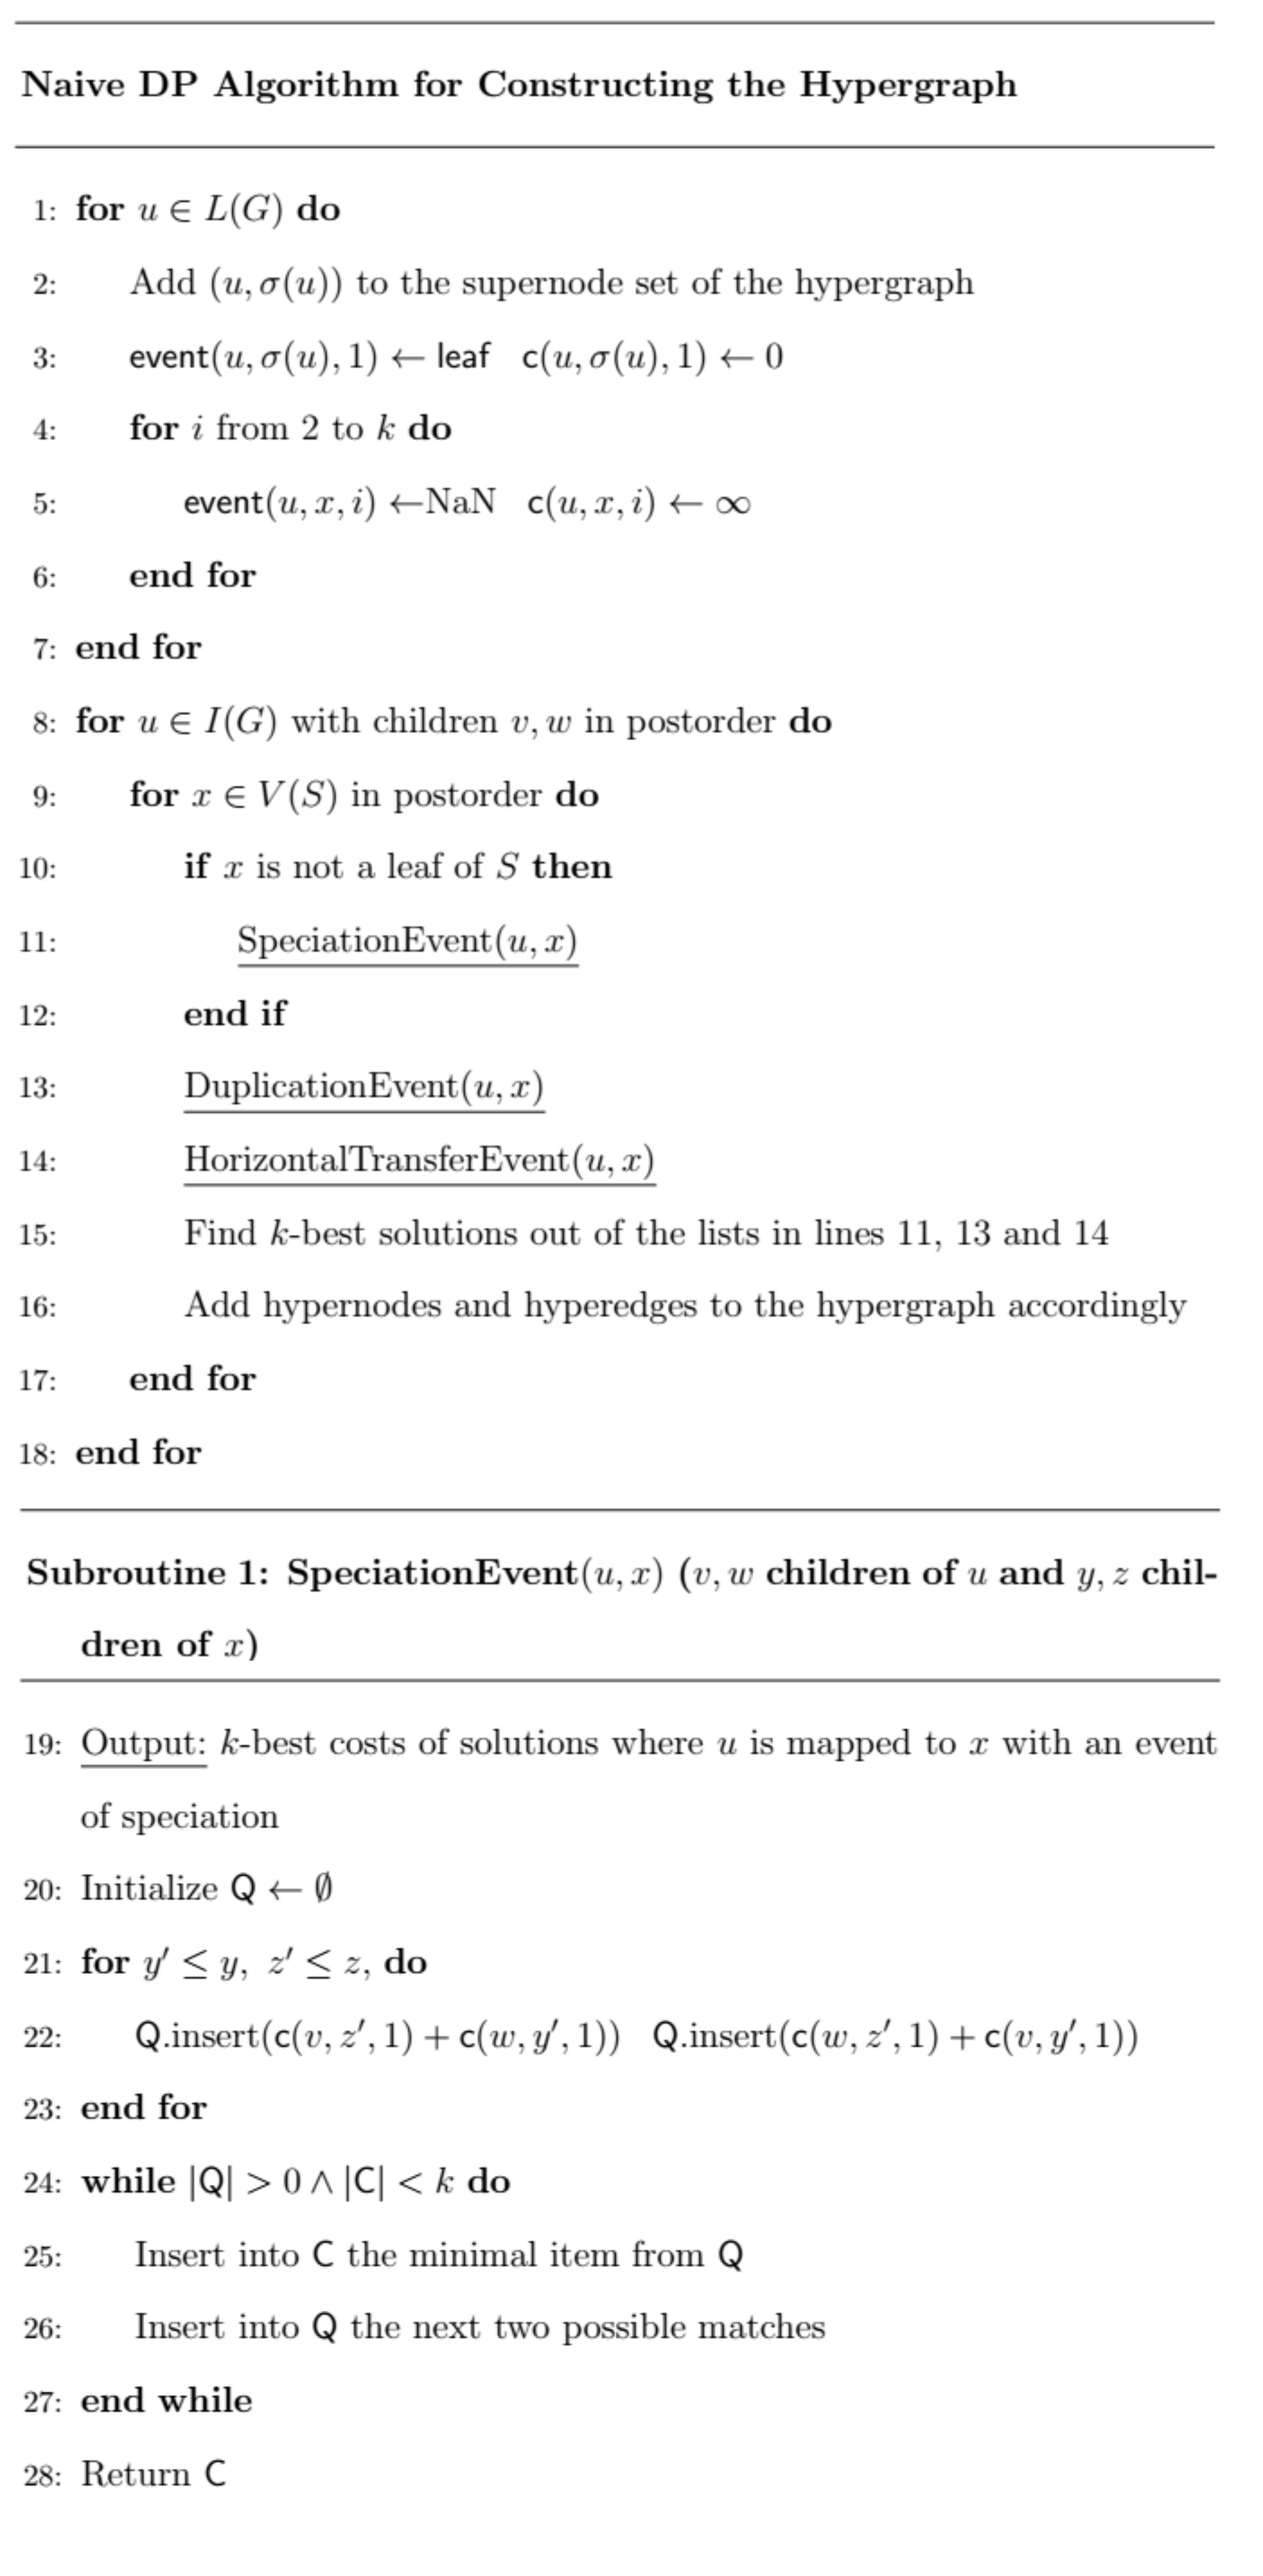}}  \caption{Psudocode of the naive version of the algorithm (first part).}
\end{center}
\end{figure}

\begin{figure}[htbp]
\begin{center}\fbox{\includegraphics[scale=0.15]{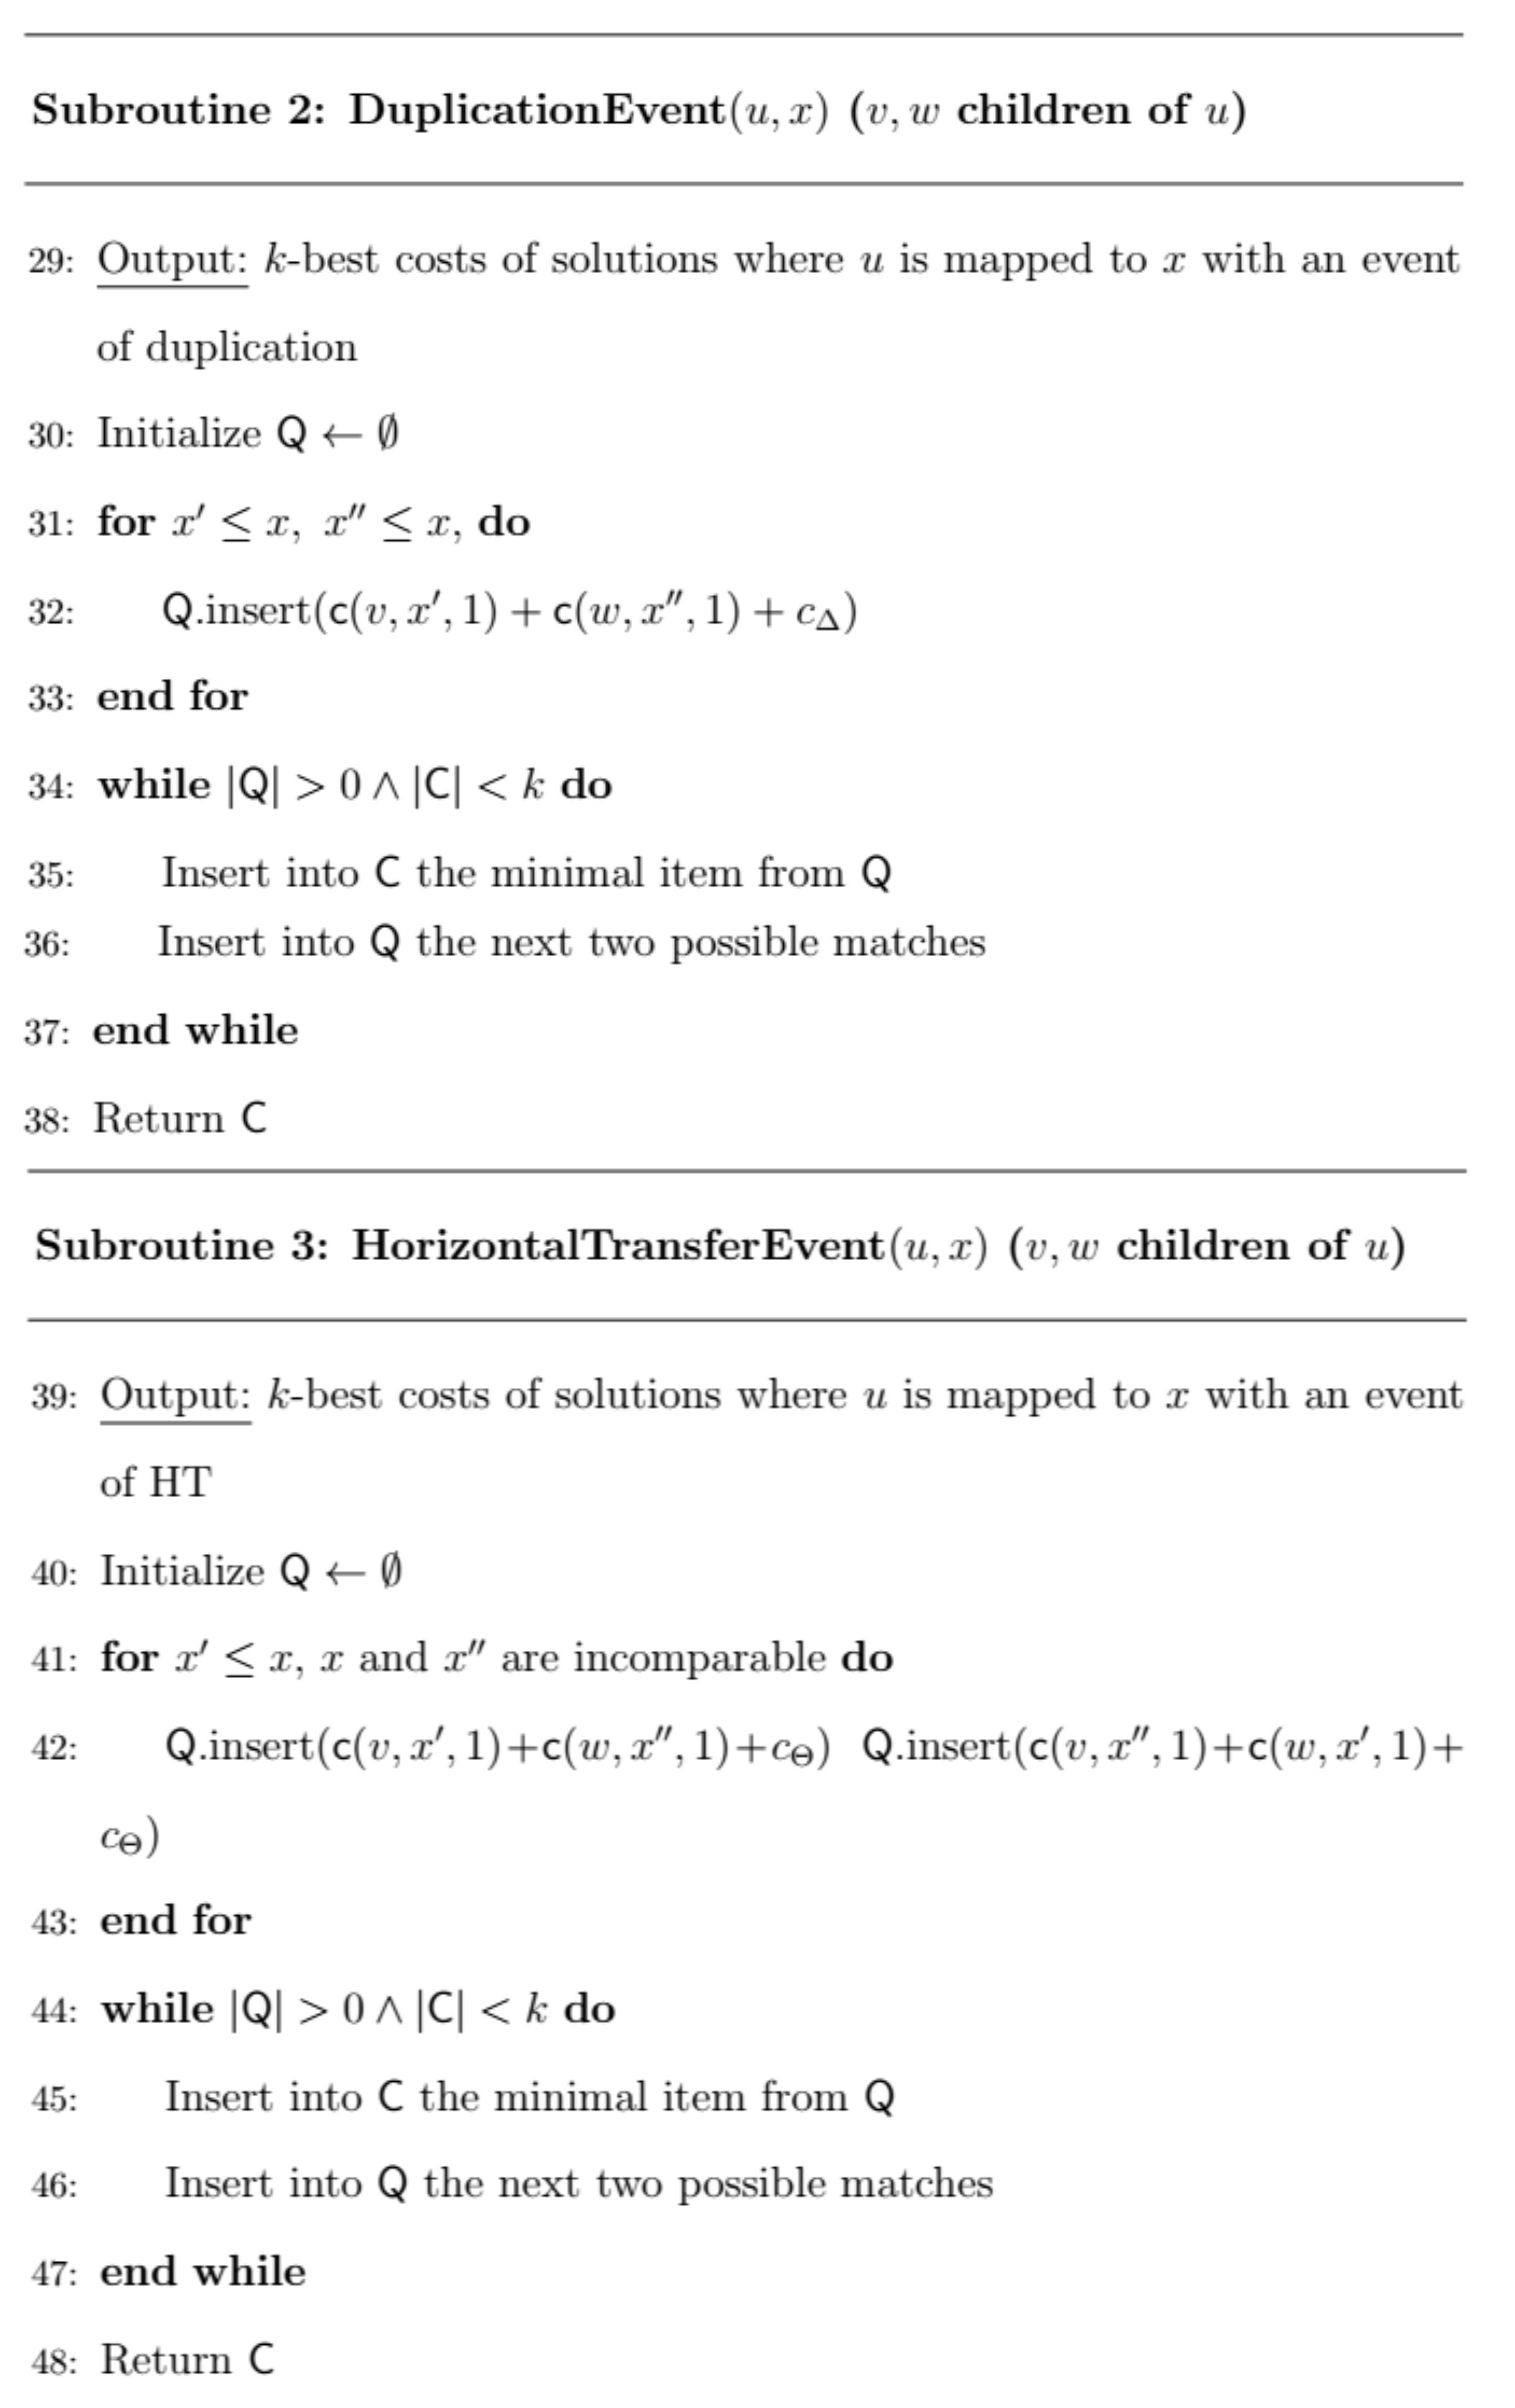}}  \caption{Psudocode of the naive version of the algorithm (second part).}
\end{center}
\end{figure}

\subparagraph*{Line 16:} After the calculation of three $k$-best lists (in Lines 11, 13 and 14) for some $u\in V(G)$ and $x\in V(S)$, we extract a list of $k$-best solutions from the single list combining these three lists. After creating a list of $k$-best solutions, we create a supernode $(u,x)$ for this list, which consists of hypernodes $(u,x,i)$ for $i\in \{ 1,\dots,k\}$. The field $\mathsf{event}(u,x,i)$ is defined by the source list (the output of SpeciationEvent, DuplicationEvent or HorizontalTransferEventFor) it was derived from. If the length of the list is shorter than $k$, then we add hypernodes with $\mathsf{event}=\mathsf{Nan}$ and $\mathsf{cost}=\infty$. For each $i\in \{ 1,\dots,k\}$, we add a hyperedge whose head is $(u,x,i)$ and whose tail is the pair of vertices that gave rise to the $i^{\mathrm{th}}$ item of the $k$-best list---that is, if the cost of $(u,x,i)$ has been derived from the costs of some two hypernodes $(v,a,j)$ and $(w,b,\ell)$, then the tail of the hyperedge is $[(v,a,j),(w,b,\ell)]$.

\subparagraph*{Line 26:} In each subroutine, we initialize a queue $\mathsf{Q}$ to contain matches corresponding to (partial) solutions at the top of  lists obtained at previous steps (see the illustrated example ahead). Next, we extract the top item of $\mathsf{Q}$, which has minimum score, say, $\mathsf{c}(v,a,1)+\mathsf{c}(w,b,1)+\mathsf{cost}$. Then, in line 26, we insert into $\mathsf{Q}$ the two next possible matches, which correspond to the scores $\mathsf{c}(v,a,2)+\mathsf{c}(w,b,1)+\mathsf{cost}$ and $\mathsf{c}(v,a,1)+\mathsf{c}(w,b,2)+\mathsf{cost}$.  Generally, upon the extraction of a top item of $\mathsf{Q}$ having some minimum score $\mathsf{c}(v,a,i)+\mathsf{c}(w,b,j)+\mathsf{cost}$, we insert (in line~26) the next two possible matches, which have scores $\mathsf{c}(v,a,i+1)+\mathsf{c}(w,b,j)+\mathsf{cost}$ and $\mathsf{c}(v,a,i)+\mathsf{c}(w,b,j+1)+\mathsf{cost}$. In case $i+1>k$, the first item is not inserted, and symmetrically for $j+1>k$.

\section{Proof of Lemma 1.} \label{sec:proof_appendix}
\begin{proof} %Exactly as in the proof of Lemma \ref{lem:naiveCorrectness}, 
We prove that for every pair of vertices $u\in V(G)$ and $x\in V(S)$, and every index $i\in\{1,\ldots,k\}$, if there exists an $i^{\mathrm{th}}$ best DLT scenario mapping the subtree of $G$ rooted in $u$ to the subtree of $S$ rooted in $x$, then the hypernode $(u,x,i)$ is inserted into the hypergraph $\cal H$ under construction with association to this scenario. In this lemma, the proof of this claim is done in conjunction with the proof that for every pair of vertices $u\in V(G)$ and $x\in V(S)$, and every index $i\in\{1,\ldots,k\}$, the following equalities hold.

\begin{itemize}
\item $\mathsf{subtreeLoss}(u,x,i)$ is the $i^{\mathrm{th}}$ best cost of a DLT scenario mapping the subtree of $G$ rooted in $u$ to some subtree of $S$ whose root is a vertex $y$ that is a descendant of $x$, with additional cost of one loss per each edge in the path from $x$ to $y$.
\item $\mathsf{subtree}(u,x,i)$ is the $i^{\mathrm{th}}$ best cost of a DLT scenario mapping the subtree of $G$ rooted in $u$ to some subtree of $S$ whose root is a vertex $y$ that is a descendant of $x$.
\item $\mathsf{incomp}(u,x,i)$ is the $i^{\mathrm{th}}$ best cost of a DLT scenario mapping the subtree of $G$ rooted in $u$ to some subtree of $S$ whose root is a vertex $y$ that is incomparable to $x$.
\end{itemize}

The proof is by induction on the order of computation. \\In particular, $\mathsf{table}_1(u_1,x_1)<\mathsf{table}_2(u_2,x_2)$ where $\mathsf{table}_1,\mathsf{table}_2\in\{\mathsf{c},\\ \mathsf{subtreeLoss},\mathsf{subtree},\mathsf{incomp}\}$ if one of the following conditions holds:
\begin{itemize}
\item $u_1$ is visited before $u_2$ in the postorder traversal of $G$.
\item $u_1=u_2$, $\mathsf{table}_1,\mathsf{table}_2\in\{\mathsf{c},\mathsf{subtreeLoss},\mathsf{subtree}\}$, and $x_1$ is visited before $x_2$ in the {\em postorder} traversal~of~$S$.
\item $u_1=u_2$, $x_1=x_2$, $\mathsf{table}_1=\mathsf{c}$ and $\mathsf{table}_2\in \{\mathsf{subtreeLoss},\mathsf{subtree}\}$.
\item $u_1=u_2$, $\mathsf{table}_1\in \{\mathsf{subtreeLoss},\mathsf{subtree}\}$ and $\mathsf{table}_2=\mathsf{incomp}$.
\item $u_1=u_2$, $\mathsf{table}_1=\mathsf{table}_2=\mathsf{incomp}$, and $x_1$ is visited before $x_2$ in the {\em preorder} traversal of $S$.
\end{itemize}

The basis of the induction comprises of the computation of hypernodes of the form $(u,x,i)$ where $u\in L(G)$. To prove its correctness, consider such a hypernode $(u,x,i)$. If $i=1$ and $x=\sigma(u)$, then the algorithm inserts the hypernode $(u,x,1)$, assigning it a score of $0$, and setting the remaining fields as follows: $\mathsf{subtreeLoss}=0$ , $\mathsf{subtree}=0$ and $\mathsf{event=leaf}$; else, if $i=1$ and $x\geq_S \sigma(u)$, then the algorithm inserts the hypernode $(u,x,1)$, assigning it a score of $0$ and setting the remaining fields as follows: $\mathsf{subtreeLoss}=c_{\mathsf{Loss}}\cdot d_S(x,\sigma(u))$, $\mathsf{subtree}=0$ and $\mathsf{event=leaf}$; otherwise, the algorithm does not insert the hypernode---more precisely, it inserts a place-holder (whose event is NaN) with score $\infty$ and $\mathsf{subtree}$ value $\infty$. In both cases, $\mathsf{incomp}$ value remains $\infty$ as in its creation. The correctness of these operations directly follows from the definitions of $\mathsf{subtreeLoss}$, $\mathsf{subtree}$ and $\mathsf{incomp}$, and the fact that the only possible DLT scenario in this case maps $u$ to an ancestor of $\sigma(u)$, and the score of this match is $0$ in case losses are not counted, or with the additional loss costs otherwise.

For the inductive step, we consider some pair of vertices $u\in I(G)$ and $x\in V(S)$ along with a table $\mathsf{table}\in\{\mathsf{c},\mathsf{subtreeLoss},\mathsf{subtree},\mathsf{incomp}\}$, and prove that the values in $\mathsf{table}$ of the supernode $(u,x)$ are computed correctly.  For the inductive assumption,  suppose that for every triple $(\mathsf{table}',u',x')$ ordered before $(\mathsf{table},u,x)$, the values in $\mathsf{table}'$ of $(u',x')$ have already been computed~correctly.

First, consider the case where $\mathsf{table}=\mathsf{subtreeLoss}$. By the pseudocode, $\mathsf{subtreeLoss}(u,x)$ consists of the $k$-best scores from the lists $\mathsf{c}(u,x),\\ \mathsf{subtreeLoss}(u,y)+c_{\mathsf{Loss}}$ (if $x$ is not a leaf) and $\mathsf{subtree}(u,z)+c_{\mathsf{Loss}}$ (if $x$ is not a leaf). Observe that these three lists have already been computed. Thus, by the inductive hypothesis, $\mathsf{c}(u,x)$ consists of the scores of the $k$-best DLT scenarios mapping the subtree of $G$ rooted in $u$ to the subtree of $S$ rooted in $x$ (where $u$ and $x$ are matched to each other), $\mathsf{subtreeLoss}(u,y)$ consists of the scores of the $k$-best DLT scenarios mapping the subtree of $G$ rooted in $u$ to the subtree of $S$ rooted in some descendant of $y$ (if $x$ is not a leaf), with additional loss cost for each edge in the path from $y$ to $\gamma(u)$, and $\mathsf{subtree}(u,z)$ consists of the scores of the $k$-best DLT scenarios mapping the subtree of $G$ rooted in $u$ to the subtree of $S$ rooted in some descendant of $z$ (if $x$ is not a leaf), with additional loss cost for each edge in the path from $z$ to $\gamma(u)$. Notice that a DLT scenario maps the subtree of $G$ rooted in $u$ to the subtree of $S$ rooted in some $x\geq_S y$ with additional cost of one loss for each edge in the path from $x$ to $y$, if and only if it is a DLT scenario that maps the subtree of $G$ rooted in $u$ to one of the following subtrees: {\em (i)} the subtree of $S$ rooted in $x$ (where $u$ and $x$ are matched), with no additional loss cost; {\em (ii)} a subtree of $S$ rooted in some descendant of $y$ (if $x$ is not a leaf), with one additional loss cost for the edge $(x,y)$; {\em (iii)} a subtree of $S$ rooted in some descendant of $z$ (if $x$ is not a leaf) with one additional loss cost for the edge $(x,z)$. Thus, it follows that $\mathsf{subtreeLoss}(u,x)$ is computed correctly.

Second, consider the case where $\mathsf{table}=\mathsf{subtree}$. By the pseudocode, $\mathsf{subtree}(u,x)$ consists of the $k$-best scores from the lists $\mathsf{c}(u,x), \mathsf{subtree}(u,y)$ (if $x$ is not a leaf) and $\mathsf{subtree}(u,z)$ (if $x$ is not a leaf). Observe that these three lists have already been computed. Thus, by the inductive hypothesis, $\mathsf{c}(u,x)$ consists of the scores of the $k$-best DLT scenarios mapping the subtree of $G$ rooted in $u$ to the subtree of $S$ rooted in $x$ (where $u$ and $x$ are matched to each other), $\mathsf{subtree}(u,y)$ consists of the scores of the $k$-best DLT scenarios mapping the subtree of $G$ rooted in $u$ to the subtree of $S$ rooted in some descendant of $y$ (if $x$ is not a leaf), and $\mathsf{subtree}(u,z)$ consists of the scores of the $k$-best DLT scenarios mapping the subtree of $G$ rooted in $u$ to the subtree of $S$ rooted in some descendant of $z$ (if $x$ is not a leaf). Notice that a DLT scenario maps the subtree of $G$ rooted in $u$ to the subtree of $S$ rooted in some descendant of $x$ if and only if it is a DLT scenario that maps the subtree of $G$ rooted in $u$ to one of the following subtrees: {\em (i)} the subtree of $S$ rooted in $x$ (where $u$ and $x$ are matched); {\em (ii)} a subtree of $S$ rooted in some descendant of $y$ (if $x$ is not a leaf); {\em (iii)} a subtree of $S$ rooted in some descendant of $z$ (if $x$ is not a leaf). Thus, it follows that $\mathsf{subtree}(u,x)$ is computed correctly.

Third, consider the case where $\mathsf{table}=\mathsf{incomp}$. By the pseudocode, if $x$ is the root of $S$, then $\mathsf{incomp}(u,x)$ does not contain any item (having score different from $\infty$) as in its creation, which is correct because in this case, there exists no vertex incomparable to $x$ and hence we cannot map one of the children of $u$ as required in the definition of the DLT scenarios that correspond to $\mathsf{incomp}(u,x)$.  Therefore, now suppose that $x$ is not the root of $S$, and let $p$ denote the parent of $x$ in $S$, and $s$ denote the sibling of $x$ in $S$ (i.e.~the other child of $p$ in $S$). Then, by the pseudocode, $\mathsf{incomp}(u,x)$ consists of the $k$-best scores from the lists $\mathsf{incomp}(u,p)$ and $\mathsf{subtree}(u,s)$. Observe that these two lists have already been computed. Thus, by the inductive hypothesis, $\mathsf{incomp}(u,p)$ consists of the scores of the $k$-best DLT scenarios mapping the subtree of $G$ rooted in $u$ to the subtree of $S$ rooted in some vertex incomparable to $p$, and $\mathsf{subtree}(u,s)$ consists of the scores of the $k$-best DLT scenarios mapping the subtree of $G$ rooted in $u$ to the subtree of $S$ rooted in some descendant of $s$. Notice that a DLT scenario maps the subtree of $G$ rooted in $u$ to a subtree of $S$ rooted in some vertex incomparable to $x$ if and only if it is a DLT scenario that maps the subtree of $G$ rooted in $u$ to one of the following subtrees: {\em (i)} a subtree of $S$ rooted in some vertex incomparable to $p$; {\em (ii)} a subtree of $S$ rooted in some descendant of $s$. Thus, it follows that $\mathsf{incomp}(u,x)$ is computed correctly.

Fourth, consider the (last) case where $\mathsf{table}=\mathsf{c}$. By line 31 of the pseudocode, $\mathsf{c}(u,x)$ consists of the $k$-best scores from the lists $p_\Sigma(u,x)$, $p_\Delta(u,x)$  and $p_\Theta(u,x)$.  Thus, to prove the correctness of the computation of $\mathsf{c}(u,x)$, it suffices to prove that the following statement holds: $p_\Sigma(u,x)$, $p_\Delta(u,x)$  and $p_\Theta(u,x)$ consist of $k$-best DLT scenarios mapping the subtree of $G$ rooted in $u$ to the subtree of $S$ rooted in $x$ under the constraint that the event corresponding to the matching of $u$ and $x$ is speciation, duplication and horizontal transfer, respectively.

Towards the proof of the statement, consider the list $p_\Sigma(u,x)$. If $x\in L(S)$, then because $u\in I(G)$, there does not exist a DLT scenario mapping the subtree of $G$ rooted in $u$ to the subtree of $S$ rooted in $x$ under the constraint that the event corresponding to the matching of $u$ and $x$ is speciation, and hence the assignment of $\infty$ to every element $p_\Sigma(u,x,i)$ of the list is correct. Now, suppose that $x\in I(S)$. Then, by the pseudocode, $p_\Sigma(u,x)$ consists of the $k$-best scores present in the following multisets: 
\begin{itemize}
\item $\{\mathsf{subtreeLoss}(v,y,j)+\mathsf{subtreeLoss}(w,z,r)~|~1\leq j,r\leq k\}$ and 
\item $\{\mathsf{subtreeLoss}(w,y,j)+\mathsf{subtreeLoss}(v,z,r)~|~1\leq j,r\leq k\}$. 
\end{itemize}
Observe that the lists $\mathsf{subtreeLoss}(v,y),\mathsf{subtreeLoss}(w,z)$, $\mathsf{subtreeLoss}(w,y)$ and $\mathsf{subtreeLoss}(v,z)$ have already been computed.  By the definition of $\mathsf{Loss}_{\alpha}(u)$ when the event occurred in $u$ is speciation,  $\mathsf{Loss}_{\alpha}(u)=|d_S (x, \gamma (v))-1|+|d_S (x, \gamma (w))-1|=d_S (y, \gamma (w))+d_S (z, \gamma (v))$ in case $\gamma(w)\leq_S y$, and $\mathsf{Loss}_{\alpha}(u)=|d_S (x, \gamma (v))-1|+|d_S (x, \gamma (w))-1|=d_S (z, \gamma (w))+d_S (y, \gamma (v))$ otherwise.  Thus, by the inductive hypothesis, $\mathsf{subtreeLoss}(v,y)$ (resp., \\ $\mathsf{subtreeLoss}(w,z)$, $\mathsf{subtreeLoss}(w,y)$ and $\mathsf{subtreeLoss}(v,z)$) consists of the scores of the $k$-best DLT scenarios mapping the subtree of $G$ rooted in $v$ (resp., $w,w$ and $v$) to a subtree of $S$ rooted in some descendant of $y$ (resp., $z,y$ and $z$), with additional loss cost for each edge in the path from $y$ to $\gamma(v)$ (resp., $\gamma(w)$, $\gamma(w)$ and $\gamma(v)$). Notice that a DLT scenario maps the subtree of $G$ rooted in $u$ to a subtree of $S$ rooted in $x$ under the constraint that the event corresponding to the matching of $u$ and $x$ is speciation if and only if it is a DLT scenario that matches $u$ and $x$, maps the subtree of $G$ rooted in $v$ to a subtree of $S$ rooted in a descendant of one child ($y$ or $z$) of $x$, and the subtree of $G$ rooted in $w$ to a subtree of $S$ rooted in a descendant of the other child of $x$. Thus, it follows that $p_\Sigma(u,x)$ is computed correctly.

Now, consider the list $p_\Delta(u,x)$. In case $x\in I(S)$, let $y$ and $z$ denote its children. By the pseudocode, $p_\Delta(u,x)$ consists of the $k$-best scores obtained by adding $c_{\Delta}$ to the costs present in the following multisets, where only the first one is relevant in case $x\in L(S)$: 
\begin{itemize}
\item $\{\mathsf{c}(v,x,j)+ \mathsf{c}(w,x,r)~|~1\leq j,r\leq k\}$, 
\item $\{\mathsf{c}(v,x,j)+\mathsf{subtreeLoss}(w,z,r)~|~1\leq j,r\leq k\}+c_{\mathsf{Loss}}$,
\item $\{\mathsf{c}(w,x,j)+\mathsf{subtreeLoss}(v,y,r)~|~1\leq j,r\leq k\}+c_{\mathsf{Loss}}$, 
\item $\{\mathsf{c}(v,x,j)+\mathsf{subtreeLoss}(w,y,r)~|~1\leq j,r\leq k\}+c_{\mathsf{Loss}}$,
\item $\{\mathsf{c}(w,x,j)+\mathsf{subtreeLoss}(v,z,r)~|~1\leq j,r\leq k\}+c_{\mathsf{Loss}}$,
\item $\{\mathsf{subtreeLoss}(v,y,j)+\mathsf{subtreeLoss}(w,z,r)~|~1\leq j,r\leq k\}+2c_{\mathsf{Loss}}$, 
\item $\{\mathsf{subtreeLoss}(w,y,j)+\mathsf{subtreeLoss}(v,z,r)~|~1\leq j,r\leq k\}+2c_{\mathsf{Loss}}$, 
\item $\{\mathsf{subtreeLoss}(v,y,j)+\mathsf{subtreeLoss}(w,y,r)~|~1\leq j,r\leq k\}+2c_{\mathsf{Loss}}$ and 
\item $\{\mathsf{subtreeLoss}(v,z,j)+\mathsf{subtreeLoss}(w,z,r)~|~1\leq j,r\leq k\}+2c_{\mathsf{Loss}}$. 
 \end{itemize}
Observe that the lists $\mathsf{c}(v,x), \mathsf{c}(w,x),\mathsf{subtreeLoss}(w,y)$, $\mathsf{subtreeLoss}(v,z)$, \\$\mathsf{subtreeLoss}(w,z)$ and $\mathsf{subtreeLoss}(v,y)$ have already been computed. By the definition of $\mathsf{Loss}_\alpha(u)$ when the event occurred in $u$ is duplication, $\mathsf{Loss}_\alpha(u)=d_S (x, \gamma (v))+d_S (x, \gamma (w))$. If $v$ (resp. $w$) is mapped to $x$ and $w$ (resp. $v$) is mapped to a subtree of rooted in $y$ or $z$, it holds that $\mathsf{Loss}_\alpha(u)=d_S (y, \gamma (w))+1$ (resp. $\mathsf{Loss}_\alpha(u)=d_S (y, \gamma (v))+1$, $\mathsf{Loss}_\alpha(u)=d_S (z, \gamma (w))+1$ and $\mathsf{Loss}_\alpha(u)=d_S (z, \gamma (v))+1$). If both $v$ and $w$ are mapped to $x$, $\mathsf{Loss}_\alpha(u)=0$, and if $v$ (resp. $w$) is mapped to $y$ or $z$ and $w$ (resp. $v$) is mapped to $y$ or $z$, it holds that $\mathsf{Loss}_\alpha(u)=d_S (y, \gamma (v))+d_S (z, \gamma (w))+2$ (resp. $\mathsf{Loss}_\alpha(u)=d_S (y, \gamma (v))+d_S (z, \gamma (w))+2$, $\mathsf{Loss}_\alpha(u)=d_S (y, \gamma (v))+d_S (v, \gamma (w))+2$, $\mathsf{Loss}_\alpha(u)=d_S (z, \gamma (v))+d_S (z, \gamma (w))+2$, $\mathsf{Loss}_\alpha(u)=d_S (z, \gamma (v))+d_S (z, \gamma (w))+2)$. Thus, by the inductive hypothesis, we have that {\em (i)} $\mathsf{c}(v,x)$ (resp. $\mathsf{c}(w,x)$) consists of the scores of the $k$-best DLT scenarios mapping the subtree of $G$ rooted in $v$ (resp. $w$) to the subtree of $S$ rooted in $x$, and {\em (ii)} $\mathsf{subtreeLoss}(v,y)$ (resp. $\mathsf{subtreeLoss}(w,z)$, $\mathsf{subtree}(w,y)$ and $\mathsf{subtreeLoss}(v,z)$) consists of the scores of the $k$-best DLT scenarios mapping the subtree of $G$ rooted in $v$ (resp. $w,w$ and $v$) to the subtree of $S$ rooted in some descendant of $y$ (resp. $z,y$ and $z$) with additional loss cost for each edge in the path from $y$ to $\gamma(v)$ (resp. $\gamma(w),\ \gamma(w)$ and $\gamma(v)$). Notice that a DLT scenario maps the subtree of $G$ rooted in $u$ to a subtree of $S$ rooted in $x$ under the constraint that the event corresponding to the matching of $u$ and $x$ is duplication if and only if it is a DLT scenario that matches $u$ and $x$, maps the subtree of $G$ rooted in $v$ to a subtree of $S$ rooted in a descendant of $x$ (which can be $x$ itself), and the subtree of $G$ rooted in $w$ to a subtree of $S$ rooted in a descendant of $x$ (which can be $x$ itself). Thus, it follows that $p_\Delta(u,x)$ is computed correctly.

Lastly, consider the list $p_\Theta(u,x)$. If $x$ is the root of $S$, then there does not exist a DLT scenario mapping the subtree of $G$ rooted in $u$ to the subtree of $S$ rooted in $x$ under the constraint that the event corresponding to the matching of $u$ and $x$ is horizontal transfer (because there is no vertex incomparable to $x$ to whom one of the children of $u$ should be mapped), and hence it is correct that each element $p_\Theta(u,x,i)$ remains with the assignment of $\infty$ as it was created. Now, suppose that $x$ is not the root of $S$. Then, by the pseudocode, $p_\Theta(u,x)$ consists of the $k$-best scores present in the following multisets: 
\begin{itemize}
\item $\{\mathsf{subtreeLoss}(v,x,j)+\mathsf{incomp}(w,x,r)~|~1\leq j,r\leq k\}$ and
\item $\{\mathsf{subtreeLoss}(w,x,j)+\mathsf{incomp}(v,x,r)~|~1\leq j,r\leq k\}$. 
\end{itemize}
Observe that the lists $\mathsf{subtreeLoss}(v,x),\mathsf{subtreeLoss}(w,x)$, $\mathsf{incomp}(w,x)$ and $\mathsf{incomp}(v,x)$ have already been computed. By the definition of $\mathsf{Loss}_\alpha(u)$ when $(u,w)\in \Xi$ , $\mathsf{Loss}_\alpha(u)=d_S (x, \gamma (v))$. Thus, by the inductive hypothesis, we have that {\em (i)} $\mathsf{subtreeLoss}(v,x)$ (resp. $\mathsf{subtreeLoss}(w,x)$) consists of the scores of the $k$-best DLT scenarios mapping the subtree of $G$ rooted in $v$ (resp. $w$) to a subtree of $S$ rooted in some descendant of $x$ (which can be $x$ itself), with additional loss cost for each edge in the path from $x$ to $\gamma(v)$ (resp. $\gamma(w)$). {\em (ii)} $\mathsf{incomp}(v,x)$ (resp. $\mathsf{incomp}(w,x)$) consists of the scores of the $k$-best DLT scenarios mapping the subtree of $G$ rooted in $v$ (resp. $w$) to a subtree of $S$ rooted in some vertex incomparable to $x$. Notice that a DLT scenario maps the subtree of $G$ rooted in $u$ to a subtree of $S$ rooted in $x$ under the constraint that the event corresponding to the matching of $u$ and $x$ is horizontal transfer if and only if it is a DLT scenario that matches $u$ and $x$, maps the subtree of $G$ rooted in one of the children of $u$ ($v$ or $w$) to a subtree of $S$ rooted in a descendant of of $x$ (which can be $x$ itself), and the subtree of $G$ rooted in the other child of $u$ to a subtree of $S$ rooted in a vertex incomparable to $x$.   Thus, it follows that $p_\Sigma(u,x)$ is computed correctly.
\end{proof}

 \end{document}
